# Supplementary material for: Hamiltonian Quantum Generative Adversarial Networks
Source: arXiv:2211.02584 source file (2024-07-08)
Supplement: Supplementary file 1 [file supplemental_simulations.tex]

\documentclass{article}
\usepackage[utf8]{inputenc}

\documentclass{article}
\usepackage[utf8]{inputenc}
\usepackage[margin=3cm]{geometry}
\usepackage{amsmath, amssymb, amsthm}
\usepackage{subfig}
\usepackage{graphicx}
\usepackage{braket}
\DeclareMathOperator{\Tr}{Tr}

\newtheorem{theorem}{Theorem}
\newtheorem{lemma}{Lemma}
\newtheorem{remark}{Remark}

\usepackage{xcolor}
\colorlet{linkequation}{blue}
\usepackage[colorlinks]{hyperref}

\newcommand*{\refeq}[1]{%
  \begingroup
    \hypersetup{
      linkcolor=linkequation,
      linkbordercolor=linkequation,
    }%
    \ref{#1}%
  \endgroup
}
\usepackage{mathtools}

\title{Supplemental Simulations}
\date{}
\begin{document}
\maketitle
\section{Time-bandwidth quantum speed limits and CRAB}
Time-bandwidth quantum speed limit (for a single control field) is described as, 
\begin{equation}\label{eq1}
    \Delta \Omega \geq \frac{D}{T\kappa_s}\log_2(1/\epsilon), 
\end{equation} where $D$ is a dimension of reachable states, $T$ is an evolution time, $\kappa$ is a bit depth, and $\epsilon$ is a precision between target and generated states. We perform a simple numerical experiment to complement the bound using CRAB.

Consider $n=3$-qubit systems of $H(t) = -\sum_{i=1}^{n-1} Z_iZ_{i+1} + f(t) (\sum_{i=1}^n X_i + Z_i)$, where $f(t)$ is a time-dependent control field to be optimized (Thus we only have a single control field to make it easy to compare with the case of Eq.\eqref{eq1}). We start from $\ket{\psi_0} = \ket{111}$ and aim to generate the GHZ state. We set $T=10$ and target fidelity to be $0.999$: RHS of Eq.\eqref{eq1} becomes $\approx 32/(10\kappa_s)$. $\kappa_s = \log_2 (1+\Delta \gamma / \delta \gamma)$ in principle can be infinitely huge if $\delta \gamma = 0$, but numerically $\kappa_s$ roughly lies between $4 \leq \kappa_s \leq 30$. This implies that the bandwidth of $f(t)$ should roughly satisfy $\Delta \Omega \gtrsim 0.8$ to get $0.999$ fidelity (assuming $\kappa_s \approx 4$). 

We used CRAB method to optimize the control field, where the ansatz of the method is a sum of $20$ fourier series with frequencies randomly chosen between $[0, w_{\max}]$. Numbers of iterations are set to be $30000$ to make sure the algorithm converges, and amplitudes of the control field are bounded by $\pm 2$. 

For each value of $w_{\max}$, we run $5$ distinct optimizations and report statistics of infidelity in Fig \ref{fig:crab1}. As expected, when $0.8 \gtrsim \Delta \Omega$, the generated state can never reach $0.999$ fidelity, and infidelity decreases as $w_{\max}$ increases. (Note that numerical results in the graph imply that the bound might not be tight, which is expected, as $ \Delta \Omega \approx 1$ still does not reach to $0.999$)

\begin{figure}[h]
    \centering
    \includegraphics[width=7.0cm]{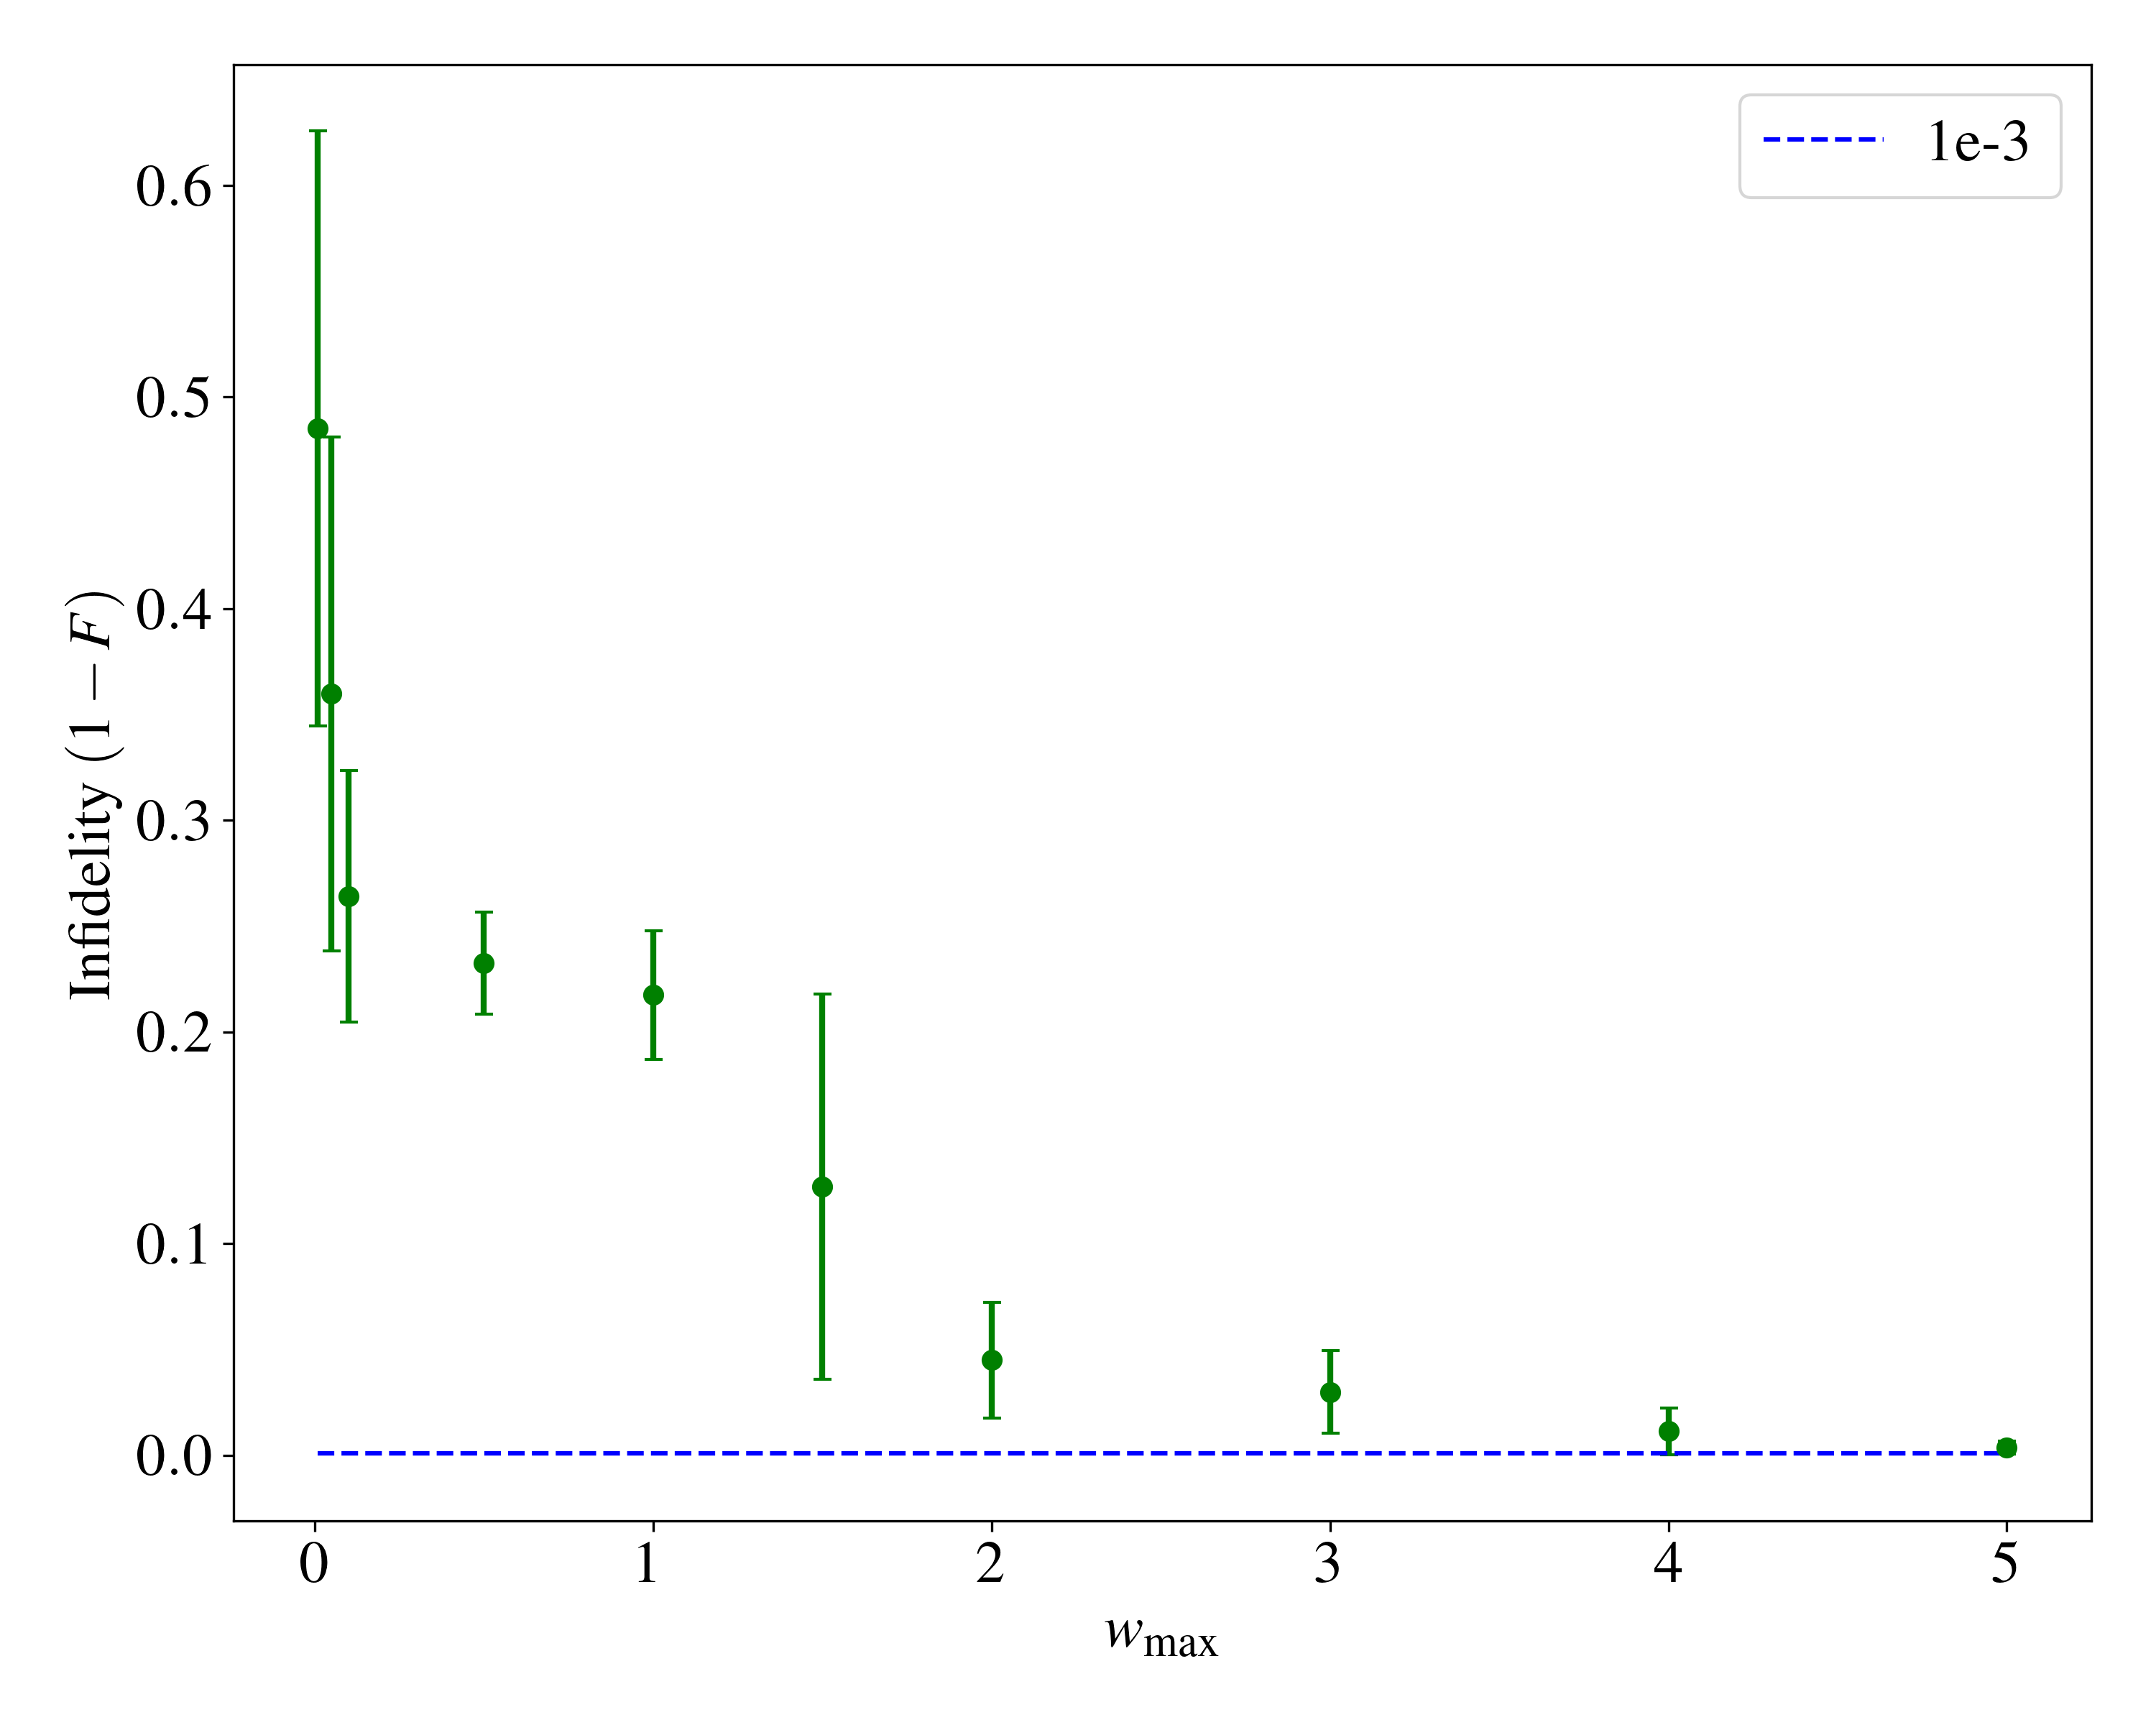}
    \caption{{Infidelity vs $w_{\max} = 0.01, 0.05, 0.1, 0.5, 1, 1.5, 2, 3, 4, 5$}. The blue dashed line indicates where fidelity = $0.999$.}
    \label{fig:crab1}
\end{figure}

\end{document}
